# Supplementary material for: High Tension Lines: Predicting robustness of high-voltage power-grids to cascading failure using network embedding
Source: arXiv:2105.13224 source file (2021-05-27)
Supplement: Supplementary file 1 [file Appendix.pdf]

# Appendix

Jonathan Bourne

February 2021

## A Parametrising $k$ with $k_{\text{range}}$ and $k_{\text{min}}$

To test whether the parametrisation of $k$ in terms of its minimum value and range have an effect on the final embedding or distribution of the embedded values 9 different parametrisations of $k$ will embedded using IEEE-118 and the results compared. The $k$ values used will be all combinations of $k_{\text{min}} = \{10, 100, 1000\}$ and $k_{\text{range}} = \{10, 100, 1000\}$. As can be seen from Fig. 1, although the raw embedding values are different, when they are normalised all embedding values are the same. This is becuase the spring stiffnesses only experience a linear transformation meaning the relative spring stiffness is unchanged. As such this shows that SETSe is robust to $k$ parametrisation and so any values of $k_{\text{min}}$ and $k_{\text{range}}$ are appropriate. It should be noted that this may not be the case if the spring stiffness function were non-linear

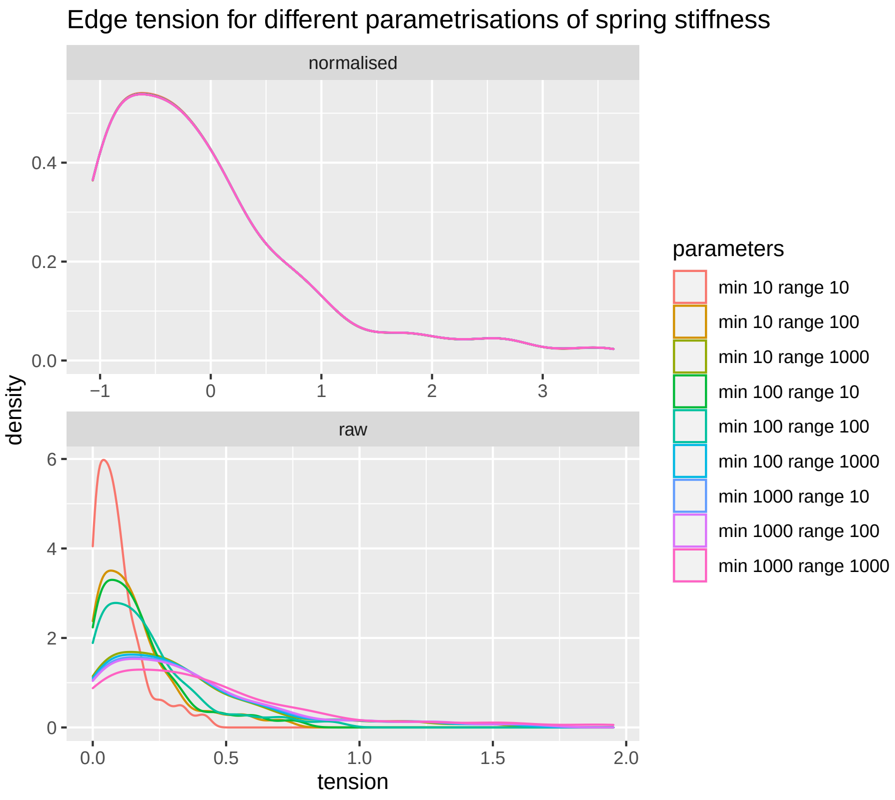


Figure 1: Although the values of$k_{\mathrm{range}}$ and $k_{\mathrm{min}}$ appear to produce different embeddings. Once the embeddings are normalised it is clear that the parametrisation has no impact on the result

# B The weakness of $\alpha$ as a robustness measure

This section will use a simple example to show the weaknesses of using $\alpha$ as a proxy for robustness, and thus the need for an alternative measure when the system is not proportionally loaded.

## B.1 Method

The network capacity ($\tau$) is the sum of the capacity of each edge, $\tau = \sum \alpha_i f_{i,j}$, where $f_{i,j}$ is the flow over edge $(i, j)$, and the edge tolerance for that line is $\alpha_{i,j}$. We show that SETSe and line load are better able to differentiate loading scenarios than $\alpha$ by fixing the values of system capacity and system tolerance for different line-loading scenarios and recording how the strain responds. To do this, we will use the simple network shown in Fig. 2. The total network capacity $\tau$ of the network will be 100 MW, while the generated/consumed power will be 20 MW. We will then change the capacity of the edges so that $\alpha_{a,b} f_{a,b} + \alpha_{b,c} f_{b,c} + \alpha_{b,d} f_{b,d} = 100$ and $\alpha_{i,j} \geq 1$ for all edges. The resulting values can then be plotted to show the relationship between system tolerance and strain when $\tau$ is fixed. What we will show is that SETSe and line load can differentiate between network loadings in a way that system tolerance and capacity cannot.

## B.2 Results

## B.3 The weakness of $\alpha$ as a robustness measure

Fig. 3 shows plots of the strain and line-load values for each simulation described in Section B. The $x$ axes of the plots show the relationship between the two demand arms of the network in terms of capacity: when they are equal, the position is 0.5, and when A has all the capacity above the minimum, the position is 0.875. The capacity $\tau$ of the system is held constant at 100. As the sum of the flow in the edges is 40, the network has 2.5 times more capacity than there is flow. As the figures show line plots in which the lines are coloured by the value of $\alpha$, it is clear that $\alpha$ is unable to distinguish between different loading scenarios that are clearly distinct using line load or strain. What we see is that the system tolerance groups are U-shaped, suggesting that as the tolerance of the demand edges becomes more similar, the robustness increases. This is sensible, as the overall ability of the network to withstand changes to the loading profile has increased. The strain and load of the system are minimised when $\alpha_{\mathrm{C}} = \alpha_{\mathrm{B}}$. It is worth noting that the minimum strain value occurs almost but not quite at the point when $\alpha = \frac{\tau}{\sum f_i}$, in this case 2.5.

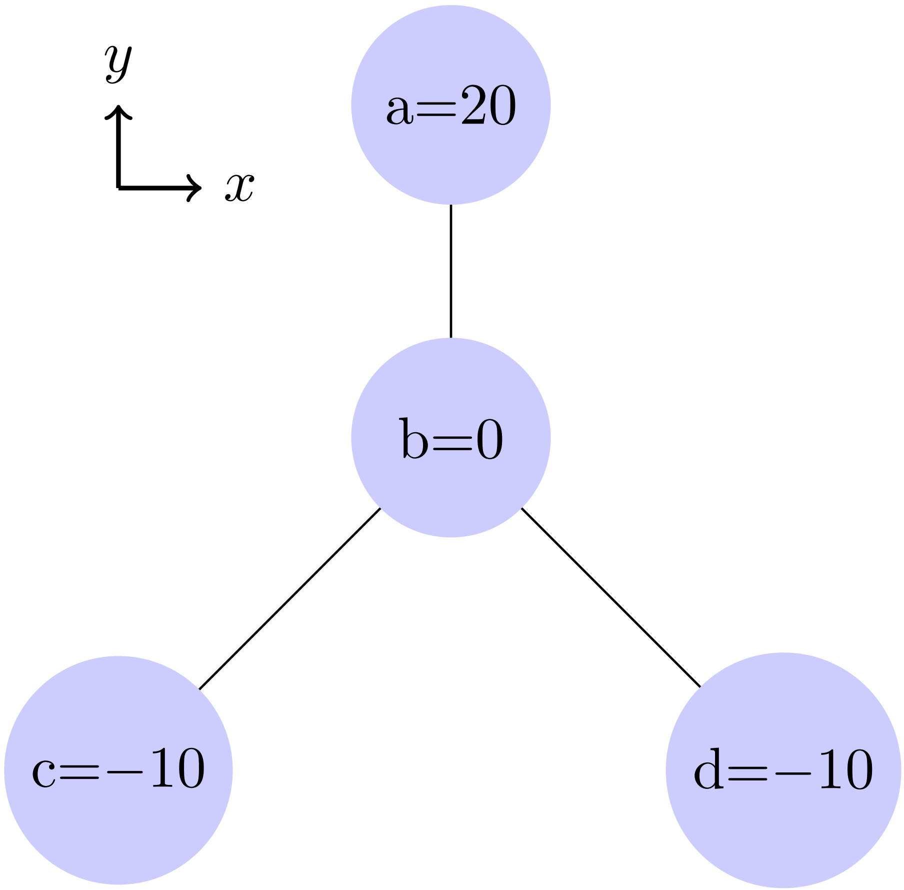


Figure 2: A network with a single generator, two demand nodes, and three edges. The network is shown in the $x$–$y$ plane.

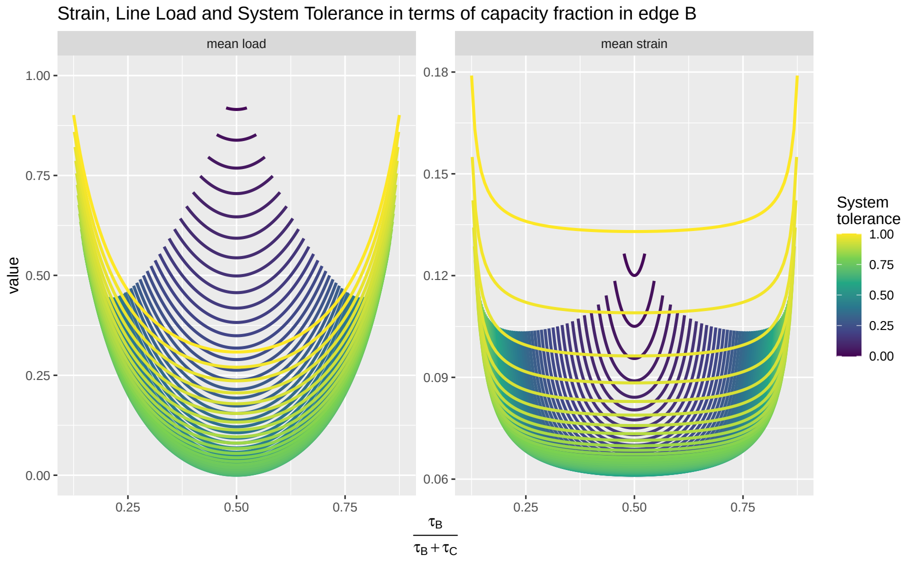


Figure 3: With a constant capacity in the system, system tolerance depends on the distribution of the capacity between edges A, B, and C. The plots show that strain and line load can differentiate between networks that have the same capacity and system tolerance.

# C Visualising the networks used

The networks described in section 2.3 are shown in Fig. 4. The networks have been embedded using SETSe and nodes are coloured by the relative elevation of the node in that network: yellow nodes are the highest and dark blue nodes are the lowest. The increasing complexity of the networks can clearly be seen, as well as their relatively different topological structures. However, the topological structure of Texas cannot be seen in this layout as the network is too large to be shown at this scale. The more complex networks also appear to have fewer loops than the simpler networks, and this is reflected in the lower clustering and betweenness values shown in Table 1.

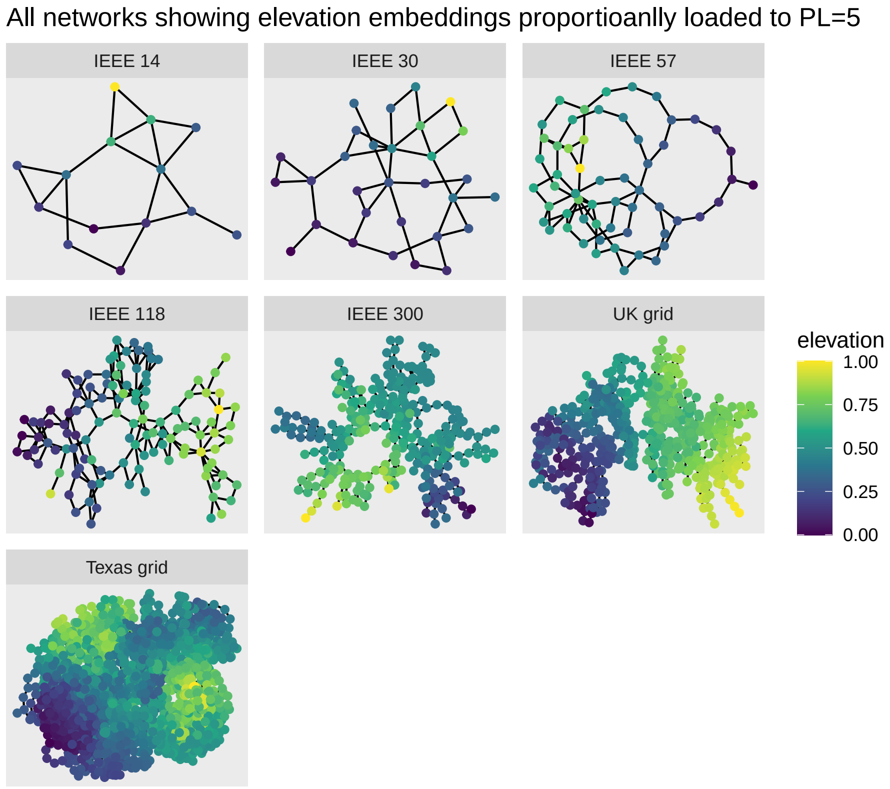


Figure 4: All the networks examined in this paper, shown with nodes coloured by SETSe elevation embedding. The layout is Kamada–Kawai [1]. The networks are proportionally loaded, with $\alpha = 5$.

# D Timeseries data

Fig. 5 shows the normal operating envelope for the power grid superimposed (shown in red) on the area covered by the tests using the redistributed load profiles (shown in black). The normal operating parameters of the network are relatively lightly loaded, and do not have too much divergence from the proportionally loaded case (shown in blue). This is an ideal scenario for the line loading measure, and is reflected in the very high correlation values. Were the network to be more heavily loaded such high values would be unlikely and SETSe may have been more accurate.

# References


[1] T. Kamada and S. Kawai. “An algorithm for drawing general undirected graphs”. In: *Information Processing Letters* 31.1 (Apr. 1989), pp. 7–15. ISSN: 0020-0190. DOI: 10.1016/0020-0190(89)90102-6.

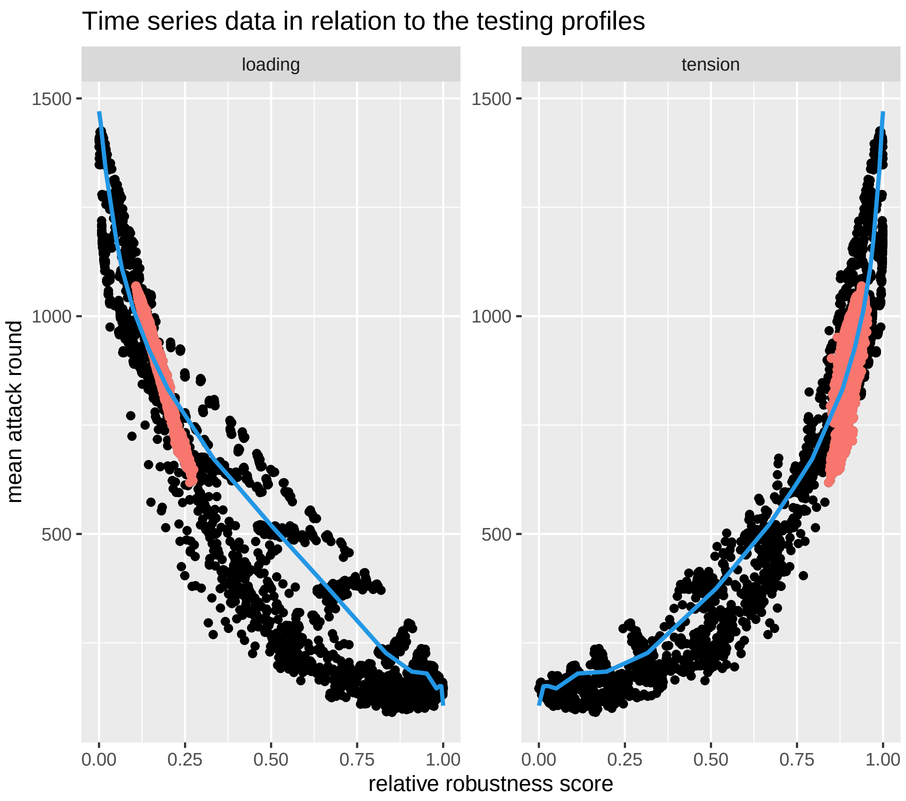


Figure 5: The time series data, shown in red, is plotted super imposed on top of the redistributed data, in black. Proportionally loaded systems are shown using the blue line. The figure shows how the normal operating envelope of the grid is in quite a small range of the total previously tested.
